# Supplementary material for: BanglaNLG and BanglaT5: Benchmarks and Resources for Evaluating Low-Resource Natural Language Generation in Bangla
Source: arXiv:2205.11081 source file (2023-02-12)
Supplement: Supplementary file 1 [file eacl2023-appendix.tex]

% This must be in the first 5 lines to tell arXiv to use pdfLaTeX, which is strongly recommended.
\pdfoutput=1
% In particular, the hyperref package requires pdfLaTeX in order to break URLs across lines.
\documentclass[11pt]{article}
% Remove the "review" option to generate the final version.
\usepackage[review]{emnlp2021}

% Standard package includes
\usepackage{times}
\usepackage{latexsym}

% For proper rendering and hyphenation of words containing Latin characters (including in bib files)
\usepackage[T1]{fontenc}
% For Vietnamese characters
% \usepackage[T5]{fontenc}
% See https://www.latex-project.org/help/documentation/encguide.pdf for other character sets

% This assumes your files are encoded as UTF8
\usepackage[utf8]{inputenc}

% This is not strictly necessary, and may be commented out,
% but it will improve the layout of the manuscript,
% and will typically save some space.
\usepackage{microtype}
\usepackage{multirow}

\usepackage{subcaption}
\usepackage{graphicx}
\usepackage{multirow}
\usepackage{enumitem}
% If the title and author information does not fit in the area allocated, uncomment the following
%
%\setlength\titlebox{<dim>}
%
% and set <dim> to something 5cm or larger.

%\title{BanglaBERT: Combating Embedding Barrier for Low-Resource Language Understanding}

\date{}

\begin{document}
\appendix
\input{appendix}
\bibliographystyle{acl_natbib}
\bibliography{anthology,eacl2023}

\end{document}
